# Supplementary material for: Self-supervised Learning with Local Contrastive Loss for Detection and Semantic Segmentation
Source: arXiv:2207.04398 source file (2022-12-08)
Supplement: Supplementary file 1 [file appendix.tex]

\onecolumn
\appendix
{
    \section*{\LARGE{Appendix}}
}

The supplemental material contains additional analysis, and ablation studies.  All these are not included in the main paper due to the space limit.

\customparagraph{Analysis on the Warping Mechanism}
In section 3, we describe that we apply warping on the log-likelihood correspondence map to get correspondence for non-integer grid locations (check Equation 4 and 5). In Table \ref{tab:pre_warp}, we pre-train another model where we apply warping on the feature space $F_{\theta}(p_t)$ using PyTorch \texttt{grid-sample} to obtain warped features on non-integer grid locations, and then calculate correspondence map. We evaluate object detection and segmentation on PASCAL VOC and COCO dataset using Faster-RCNN and mask-RCNN respectively. Even though \ours(feature-warp) still shows good performance, we get the best results when we apply warping on the log likelihood correspondence map $\text{NLL}(p_c, p_t)$.

\begin{table}[!htbp]
    \centering
    \begin{adjustbox}{max width=\linewidth}
        \begin{tabular}{c | c c c | c c c c c c}
            \toprule
            {\bf  Method}       & \multicolumn{3}{c|}{{\bf  PASCAL VOC}} & \multicolumn{6}{c}{\bf  COCO}                                                                                                                                                                                    \\
                                & {\bf $\text{AP}^b$}                    & {\bf $\text{AP}^b_{50}$}      & {\bf $\text{AP}^b_{75}$} & {\bf $\text{AP}^b$} & {\bf $\text{AP}^b_{50}$} & {\bf $\text{AP}^b_{75}$} & {\bf $\text{AP}^m$} & {\bf $\text{AP}^m_{50}$} & {\bf $\text{AP}^m_{75}$} \\
            \midrule
            \ours(feature-warp) & -                  \\
            \ours         &  -                   \\
            \bottomrule
        \end{tabular}
    \end{adjustbox}
    \caption{{{\bf Experiments with our method when warping on the feature space.} The models are pretrained on the COCO dataset for 800 epochs with the same settings. Warping on the log likelihood is better than warping on the features. }}
    \label{tab:pre_warp}
\end{table}

% \todo{COCO 2x results}

\begin{table}[!htbp]
    \centering
    % \caption{\small \textbf{COCO object detection}}
    % \label{tab:coco_retina}
    \begin{minipage}{0.6\textwidth}
        \begin{tabular}{l c c c c}
            \toprule
            {\bf Method}                                  & {\bf Pretrain Epoch} & {\bf $\text{AP}$} & {\bf $\text{AP}_{50}$} & {\bf $\text{AP}_{75}$} \\
            \midrule
            Scratch                                       & -                    & 24.5              & 39.0                   & 25.7                   \\
            Supervised  \cite{he2016deepresnet}           & 90                   & 37.7              & 57.2                   & 40.4                   \\
            Moco v2   \cite{chen2020improvedmocov2}       & 200                  & 37.3              & 56.2                   & 40.4                   \\
            SimCLR v2 \cite{chen2020bigsimclrv2}          & 800                  & 37.4              & 56.5                   & 40.3                   \\
            BYOL  \cite{grill2020bootstrapbyol}           & 300                  & 35.4              & 54.7                   & 37.4                   \\
            SwAV \cite{caron2020unsupervisedswav}         & 400                  & 35.2              & 54.9                   & 37.5                   \\
            \midrule
            ReSim-FPN$^{*}$ \cite{xiao2021regionresim}    & 200                  & 38.6              & 57.6                   & 41.6                   \\
            SoCo    \cite{wei2021aligningsoco}            & 400                  & 38.3              & 57.2                   & 41.2                   \\
            SCRL    \cite{roh2021spatiallyscrl}           & 1000                 & 39.0              & 58.7                   & 41.9                   \\
            \midrule
            DetCo        \cite{xie2021detco}              & 800                  & 38.4              & 57.8                   & 41.2                   \\
            DenseCL$^{*}$       \cite{wang2021densecl}    & 200                  & 37.6              & 56.6                   & 40.2                   \\
            PixPro$^{*}$    \cite{xie2021propagatepixpro} & 400                  & 38.7              & 57.5                   & 41.6                   \\
            \rowcolor{_teal3} \ours                       & 400                  & \bf40.6           & \bf60.4                & \bf43.6                \\
            \bottomrule
        \end{tabular}
    \end{minipage}
    \hspace{0.01\linewidth}
    \begin{minipage}{0.35\textwidth}
        \caption{\textbf{COCO object detection.} We use finetune on the COCO \texttt{train2017} set using faster-RCNN RetinaNet FPN network for 90k iterations. {\bf$^{*}$}: denotes that we perform the finetuning using publicly available checkpoints released by the authors.}
        \label{tab:coco_retina}
    \end{minipage}
\end{table}

\begin{table}[!tbp]
    \centering
    \caption{\small \textbf{Object detection and instance segmentation fine-tuned on COCO.} We use Mask R-CNN R50-FPN (1$\times$ schedule), and report bounding-box AP (AP$^{bb}$) and mask AP (AP$^{mk}$).}
    \label{tab:coco_mrcnn}
    \begin{tabular}{l c c c c c c c}
        \toprule
        \multirow{2}{*}{\bf Method}                    &
        \multirow{2}{*}{\bf \begin{tabular}[c]{c}Pretrain\\ epoch\end{tabular}} &
        \multicolumn{3}{c}{\bf Detection}              &
        \multicolumn{3}{c}{\bf Instance-seg.}                                                                                                                       \\
                                                       &      & AP$^{bb}$      & AP$^{bb}_{50}$ & AP$^{bb}_{75}$ & AP$^{mk}$      & AP$^{mk}_{50}$ & AP$^{mk}_{75}$ \\ \midrule
        Scratch                                        & -    & 31.0           & 49.5           & 33.2           & 28.5           & 46.8           & 30.4           \\
        Supervised                                     & 90   & 38.9           & 59.6           & 42.7           & 35.4           & 56.5           & 38.1           \\
        \midrule
        MoCo                                           & 200  & 38.5           & 58.9           & 42.0           & 35.1           & 55.9           & 37.7           \\
        MoCo v2                                        & 200  & 40.4           & 60.2           & 44.2           & 36.4           & 57.2           & 38.9           \\
        InfoMin                                        & 200  & 40.6           & 60.6           & 44.6           & 36.7           & 57.7           & 39.4           \\
        BYOL                                           & 300  & 40.4           & 61.6           & 44.1           & 37.2           & 58.8           & 39.8           \\
        % SwAV                                           & 400  & -              & -              & -              & -              & -              & -              \\
        VADeR                                          & 200  & 39.2           & 59.7           & 42.7           & 35.6           & 56.7           & 38.2           \\
        \midrule
        ReSim-FPN$^{T}$                                & 200  & 39.8           & 60.2           & 43.5           & 36.0           & 57.1           & 38.6           \\
        SoCo                                           & 400  & \bf43.0        & \boldsec{63.3} & \bf47.1        & 38.2           & \boldsec{60.2} & 41.0           \\
        DetCon$_{S}$                                   & 1000 & 41.8           & -              & -              & 37.4           & -              & -              \\
        DetCon$_{B}$                                   & 1000 & {42.7}         & -              & -              & 38.2           & -              & -              \\
        \midrule
        DenseCL                                        & 200  & 40.3           & 59.9           & 44.3           & 36.4           & 57.0           & 39.2           \\
        DetCo                                          & 800  & 40.1           & 61.0           & 43.9           & 36.4           & 58.0           & 38.9           \\
        InsLoc                                         & 400  & 42.0           & 62.3           & 45.8           & 37.6           & 59.0           & 40.5           \\
        PixPro                                         & 400  & 41.4           & 61.6           & 45.4           & -              & -              & -              \\
        \rowcolor{_teal3} \ours                        & 200  & 42.0           & 62.5           & 46.3           & 37.9           & 59.5           & 40.8           \\
        \rowcolor{_teal3} \ours                        & 400  & 42.5           & 62.9           & 46.7           & \boldsec{38.3} & \boldsec{60.0} & \boldsec{41.1} \\
        \rowcolor{_teal3} \ours                        & 600  & \boldsec{42.8} & \textbf{63.4}  & \boldsec{46.6} & \bf38.6        & \bf60.4        & \bf41.5        \\
        \bottomrule
    \end{tabular}
\end{table}

\begin{table}[!htbp]
    \centering
    \begin{adjustbox}{max width=\linewidth}
        \begin{tabular}{l c c p{3em} c c c}
            \toprule
            {\bf Method}               & {\bf $\text{AP}^b$} & {\bf $\text{AP}^b_{50}$} & {\bf $\text{AP}^b_{75}$} & {\bf $\text{AP}^m$} & {\bf $\text{AP}^m_{50}$} & {\bf $\text{AP}^m_{75}$} \\
            \midrule
            Scratch                    & 32.8                & 50.9                     & 35.3                     & 29.9                & 47.9                     & 32.0                     \\
            Supervised IN              & 39.7                & 59.5                     & 43.3                     & 35.9                & 56.6                     & 38.6                     \\
            BYOL IN                    & 36.9                & 57.5                     & 39.7                     & 32.4                & 53.7                     & 34.1                     \\
            \rowcolor{_teal3} \ours IN & 38.8                & 58.9                     & 41.8                     & 33.8                & 55.4                     & 35.5                     \\
            \midrule
            BYOL CC                    & 37.1                & 56.7                     & 39.9                     & 32.5                & 53.4                     & 34.3                     \\
            \rowcolor{_teal3} \ours CC & 38.7                & 58.2                     & 41.8                     & 33.6                & 54.9                     & 35.5                     \\
            \bottomrule
        \end{tabular}
    \end{adjustbox}
    % \vspace{-2mm}
    \caption{{\small {\bf COCO object detection and semantic segmentation.} We use 1$\times$ schedule to finetune on COCO \texttt{train2017} and evaluate on \texttt{val2017}.}}
    \label{tab:coco_mask_rcnn}
    % \vspace{-3mm}
    % \caption{{\small {\bf Object detection and semantic segmentation on COCO.} We use 1x schedule to finetune on COCO \texttt{train2017} and evaluate on \texttt{val2017}. For ImageNet pretrained models, \putalg improves upon BYOL by 1.9\% for detection and 1.6\% for segmentation. For COCO pretrained backbone, we outperform BYOL by 1.6\% for detection and 1.1\% for segmentation. Improvement is larger for stringent threshold AP$^{75}$. Results for $2\times$ schedule are reported in the supplementary.\todo{Remove commentary as it is already in the main text.}}}
\end{table}

\customparagraph{COCO Keypoint Estimation.} \todo{Keypoint estimation} We use Mask-RCNN (keypoint version) with ResNet50 FPN network to evaluate keypoint estimation task. We finetune on COCO \texttt{train 2017} dataset for 90k iterations. Table \ref{tab:coco_kp} shows that our method outperforms all other approaches in keypoint estimation task.
\begin{table}[!htbp]
    \centering
    \begin{minipage}{0.5\textwidth}
        \begin{adjustbox}{max width=0.9\linewidth}
            \begin{tabular}{l c c c c}
                \toprule
                {\bf Method}            & {\bf Pretrain Epoch} & {\bf $\text{AP}$} & {\bf $\text{AP}_{50}$} & {\bf $\text{AP}_{75}$} \\
                \midrule
                % Scratch                 & -                    & -                 & -                      & -                      \\
                Supervised              & 90                   & 65.7              & 87.2                   & 71.5                   \\
                Moco v2                 & 200                  & 65.9              & 86.9                   & 71.6                   \\
                BYOL                    & 300                  & 66.3              & 87.4                   & 72.4                   \\
                % \midrule
                VADeR$^{\dagger}$       & 200                  & 66.1              & 87.3                   & 72.1                   \\
                SCRL$^{\dagger}$        & 1000                 & 66.5              & 87.8                   & 72.3                   \\
                ReSim-FPN               & 200                  & 66.6              & 87.4                   & 72.8                   \\
                % SoCo                    & 400                  & -                 & -                      & -                      \\
                % \midrule
                % DetCo                   & 800                  & -                 & -                      & -                      \\
                DenseCL                 & 200                  & 66.2              & 87.3                   & 71.9                   \\
                PixPro                  & 400                  & 66.6              & \bf87.8                & 72.8                   \\
                \rowcolor{_teal3} \ours & 400                  & \bf67.2           & 87.4                   & \bf73.7                \\
                \bottomrule
            \end{tabular}
        \end{adjustbox}
    \end{minipage}
    %
    % \hspace{0.01\linewidth}
    \begin{minipage}{0.35\textwidth}
        \caption{\small \textbf{COCO keypoint estimation.} We use the publicly available ImageNet-pretrained checkpoints released by the authors and finetune on the COCO dataset with Keypoint R50-FPN network for 90k iteration. ($^{\dagger}$) denotes scores from the original papers.}
        \label{tab:coco_kp}
    \end{minipage}
\end{table}

\customparagraph{Semi-supervised Detection.}
As the full COCO dataset contains extensive annotated images for supervision, it might not always reveal the generalization ability of the network.Therefore, we also report results for semi-supervised object detection and segmentation on smaller versions of COCO training set in Table \ref{tab:coco_semi}. We report results when only 5\% and 10\% of the images (randomly sampled) are used for finetuning the mask-RCNN with FPN network. The evaluation is performed on the full \texttt{val2017} set. For the 5\% setting, our method outperforms BYOL by 1.4\% AP for the ImageNet pretrained models, and . For the 10\% setting, our method achieves improvement over BYOL by 1.8\% AP.

\begin{table}[!htbp]
    \centering
    \begin{minipage}{0.55\textwidth}
        \begin{adjustbox}{max width=\linewidth}
            \begin{tabular}{p{0.26\linewidth} c  c  c  | c c c}
                \toprule
                                        & \multicolumn{3}{c}{\bf 5\%} & \multicolumn{3}{c}{\bf 10\%}                                                                                                \\
                \cmidrule(lr){2-4} \cmidrule(lr){5-7}
                {\bf Method}            & {\bf $\text{AP}$}           & {\bf $\text{AP}_{50}$}       & {\bf $\text{AP}_{75}$} & {\bf $\text{AP}$} & {\bf $\text{AP}_{50}$} & {\bf $\text{AP}_{75}$} \\
                \midrule
                % Scratch   \\
                Supervised              & 19.2                        & 31.0                         & 20.5                   & 25.0              & 39.9                   & 26.6                   \\
                Moco v2                 & 18.2                        & 28.9                         & 19.8                   & 23.9              & 37.8                   & 25.6                   \\
                BYOL                    & 21.9                        & 36.2                         & 23.2                   & 27.1              & 43.4                   & 29.3                   \\
                DenseCL                 & -                           & -                            & -                      & 24.8              & 38.8                   & 26.8                   \\
                PixPro                  & 20.3                        & 31.4                         & 22.1                   & 25.4              & 39.5                   & 27.4                   \\
                \rowcolor{_teal3} \ours & \bf23.3                     & \bf37.4                      & \bf25.0                & \bf27.9           & \bf44.0                & \bf30.1                \\
                \bottomrule
            \end{tabular}
        \end{adjustbox}
    \end{minipage}
    \begin{minipage}{0.3\textwidth}
        \caption{{\small {\bf Semi-supervised object detection on COCO.} We use 5\% and 10\% of the training data sampled randomly from the full \texttt{train2017} set, and evaluate on the \texttt{val2017} set.}}
        % \vspace{-2mm}
        \label{tab:coco_semi}
    \end{minipage}
    % \vspace{-2mm}
\end{table}

\section{Ablations on the Warping Mechanism}
In section 3, we describe that we apply warping on the log-likelihood correspondence map to get correspondence for non-integer grid locations (check Equation 4 and 5). In Table \ref{tab:pre_warp}, we pre-train another model where we apply warping on the feature space $F_{\theta}(p_t)$ using PyTorch \texttt{grid-sample} to obtain warped features on non-integer grid locations, and then calculate correspondence map. We evaluate object detection and segmentation on PASCAL VOC and COCO dataset using Faster-RCNN and mask-RCNN respectively. Even though \ours(feature-warp) still shows good performance, we get the best results when we apply warping on the log likelihood correspondence map $\text{NLL}(p_c, p_t)$.

\begin{table}[!htbp]
    \centering
    \begin{adjustbox}{max width=\linewidth}
        \begin{tabular}{c | c c c | c c c c c c}
            \toprule
            {\bf  Method}       & \multicolumn{3}{c|}{{\bf  PASCAL VOC}} & \multicolumn{6}{c}{\bf  COCO}                                                                                                                                                                                    \\
                                & {\bf $\text{AP}^b$}                    & {\bf $\text{AP}^b_{50}$}      & {\bf $\text{AP}^b_{75}$} & {\bf $\text{AP}^b$} & {\bf $\text{AP}^b_{50}$} & {\bf $\text{AP}^b_{75}$} & {\bf $\text{AP}^m$} & {\bf $\text{AP}^m_{50}$} & {\bf $\text{AP}^m_{75}$} \\
            \midrule
            \ours(feature-warp) & 56.9                                   & 81.6                          & 63.6                     & 38.1                & 57.6                     & 41.0                     & 33.2                & 54.1                     & 35.2                     \\
            \ours               & 57.1                                   & 81.7                          & 63.4                     & 38.7                & 58.2                     & 41.8                     & 33.6                & 54.9                     & 35.5                     \\
            \bottomrule
        \end{tabular}
    \end{adjustbox}
    \caption{{{\bf Experiments with our method when warping on the feature space.} The models are pretrained on the COCO dataset for 800 epochs with the same settings. Warping on the log likelihood is better than warping on the features. }}
    \label{tab:pre_warp}
\end{table}

\section{Experiments with MoCo-v2}
In Table \ref{tab:moco}, we perform experiments for pretrained models that are trained with MoCo-v2 framework  \cite{he2020momentummoco}. We use ResNet-50 \cite{he2016deepresnet} as our backbone network.  We use the SGD optimizer with base learning rate of 0.3 for batch size 256. We train on 16 GPUs with 64 batch size per GPU for 800 epochs, and apply linear scaling for setting the learning rate. We see that our approach also works better for contrastive self-supervised learning framework. Specifically, we achieve 2.4\% improvement over vanilla MoCo pretrained model in terms of average AP for object detection using faster-RCNN, and 2.5\% mIoU improvement for segmentation using FCN ResNet50-C4 framework.

\begin{table}[!htbp]
    \centering
    \begin{adjustbox}{max width=\linewidth}
        \begin{tabular}{c | c c c | c }
            \toprule
            {\bf  Method}   & \multicolumn{4}{c}{{\bf  PASCAL VOC}}                                                                    \\
                            & {\bf $\text{AP}^b$}                   & {\bf $\text{AP}^b_{50}$} & {\bf $\text{AP}^b_{75}$} & {\bf mIoU} \\
            \midrule
            MoCo-v2 CC      & 53.8                                  & 80.4                     & 59.6                     & 65.1       \\
            \ours (MoCo-v2) & 56.2                                  & 81.5                     & 62.2                     & 67.6       \\
            \bottomrule
        \end{tabular}
    \end{adjustbox}
    \caption{{{\bf Object detection and segmentation on PASCAL VOC for COCO-pretrained models with MoCO-v2.} Both models are trained on COCO dataset for 800 epochs with similar settings. Our approach also works better for contrastive self-supervised learning framework. Object detection is performed on faster-RCNN framework and segmentation on FCN ResNet50-C4.}}
    \label{tab:moco}
\end{table}

\section{Implementation Details for Downstream Tasks with ResNet50 backbone}
For faster-RCNN and mask-RCNN on ResNet50 backbones, we use Detectron2 framework \cite{wu2019detectron2} with similar settings as \cite{wang2021densecl}. For segmentation, we use mmseg framework \cite{mmseg2020}. We use SGD optimizer with learning rate 0.01 and momentum 0.9, and weight-decay 0.0005. We use 20k schedule for VOC and 40k schedule for CityScapes and ScanNet. All the models are trained on 8 GPU with batch-size 2 per GPU.

\section{Details on Vision Transformer Backbone}
\paragraph{Pretraining} We use DINO \cite{caron2021emergingdino} self-supervised learning framework with Swin Transformer \cite{liu2021swin} backbone to evaluate our approach on vision transformer. We use Swin-T variant which has similar parameters as ResNet50, please refer to the original paper \cite{liu2021swin} for more details on the Swin Transformer backbone. We use AdamW optimizer with base learning rate of 0.0005 for batch-size 256 and weight-decay of 0.04. We pretrain the model for 300 epochs on 16 GPUs with 64 batch-size per GPU. For Swin with our approach, we set weight parameter $\alpha =0.5$. We use similar image transformations as the other experiments in the main paper for pretraining. The backbones are trained on ImageNet training set. We tried to also pretrain the backbone on COCO dataset, however, the network did not converge.
\paragraph{Object Detection and Segmentation} We use mmdetection framework \cite{mmdetection} to train and evaluate on the downstream dataset with Swin transformer backbone. For faster-RCNN and mask-RCNN, we use ResNet50-FPN variant, train the models with AdamW optimizer for learning rate 0.0001 and weight-decay 0.05 on 8 GPUs with batch-size 2 per GPU. For segmentation, we use mmseg framework \cite{mmseg2020}. We use UperNet \cite{xiao2018unifiedupernet} for segmentation on VOC, CityScapes, and ScanNet. We use AdamW optimizer with learning rate 0.00006 and weight-decay 0.01. We train on PASCAL VOC for 20k iterations, and 40k iterations on the other datasets.

% \section{Time Complexity}
% To train BYOL on COCO dataset for 800 epochs on COCO dataset, it takes around $\sim$22 hours 45 mins. To train \ours with BYOL for 800 epochs, it takes around $\sim$ 24 hours and 18 mins. We see that our approach takes only 6.8\% longer to train to additionally calculate the local correspondence loss.

\section{Results on COCO with 2x Schedule}
Table \ref{tab:coco_2x} shows results with Mask-RCNN 2x schedule on COCO dataset for ImageNet pretrained model. \ours improve over BYOL pretrained backbone by 1.7\% AP on detection and 1.2\% AP on segmentation.

\begin{table}[!htbp]
    \centering
    \begin{adjustbox}{max width=\linewidth}
        \begin{tabular}{l c c p{3em} c c c}
            \toprule
            {\bf Method}               & {\bf $\text{AP}^b$} & {\bf $\text{AP}^b_{50}$} & {\bf $\text{AP}^b_{75}$} & {\bf $\text{AP}^m$} & {\bf $\text{AP}^m_{50}$} & {\bf $\text{AP}^m_{75}$} \\
            \midrule
            BYOL IN                    & 39.6                & 59.6                     & 42.8                     & 34.5                & 56.2                     & 36.8                     \\
            \rowcolor{_teal3} \ours IN & 41.3                & 61.1                     & 44.9                     & 35.7                & 57.8                     & 37.8                     \\
            \bottomrule
        \end{tabular}
    \end{adjustbox}
    \caption{{\small {\bf COCO object detection and semantic segmentation with 2x schedule.} We use 1$\times$ schedule to finetune on COCO \texttt{train2017} and evaluate on \texttt{val2017}.}}
    \label{tab:coco_2x}
\end{table}

\subsection{Analyzing Vision Transformer Backbone}

\todo{[SUPPLEMENTAL] }
We perform experiments using a vision transformer backbone to evaluate whether our method benefits transformer pretraining. We use Swin transformer \cite{liu2021swin}, which is a hierarchical vision transformer using shifted windows. It also has a multi-scale architecture that is suitable for dense estimation tasks. For the self-supervised architecture with transformer, we use DINO \cite{caron2021emergingdino}. DINO directly predicts the output of a teacher network by a standard cross-entropy loss, without using predictor or contrastive loss. We follow similar settings for pretraining as the DINO paper \cite{caron2021emergingdino}. We do not use multi-crop transformation. We pretrain the models on ImageNet1k dataset for 300 epochs. More technical details are provided in the supplementary material.

In Table \ref{tab:swin}, we report results for the PASCAL VOC, MS COCO, CityScapes, and ScanNet datasets. For PASCAL VOC detection, we use a Faster-RCNN framework with ResNet-50 FPN backbone, and for segmentation, we use the UperNet \cite{xiao2018unifiedupernet} framework. \putalg improves detection performance by 1.6\% AP and segmentation results by 2.1\% mIoU.  For COCO object detection and instance segmentation, we use mask-RCNN with a ResNet-50 FPN backbone. Our method outperforms the baseline by 0.8\% in detection and 0.4\% in segmentation. We perform segmentation on the CityScapes and ScanNet datasets using the UperNet framework. Our approach increases the mIoU by 0.1\% for CityScapes and 1.0\% for ScanNet. More technical details about the finetuning setup are in the supplementary material. We note that the improvement for transformer is not as impressive as for the ResNet-50 backbone, which suggests that the self-supervised vision transformer might already have more spatial information in its feature representation than ResNet-50. This also aligns with the conclusion from \cite{caron2021emergingdino} that the vision transformer contains information related to scene layout in the features.

\begin{table*}[!htbp]
    \centering
    \begin{adjustbox}{max width=\linewidth}
        \begin{tabular}{l | c c c c| c c c c c c| c | c}
            \toprule
            {\bf \small Method}  & \multicolumn{4}{c|}{{\bf \small PASCAL VOC}} & \multicolumn{6}{c|}{COCO} & {\bf \small Cityscapes}  & {\bf \small ScanNet}                                                                                                                                                                       \\
                                 & {\bf $\text{AP}^b$}                          & {\bf $\text{AP}^b_{50}$}  & {\bf $\text{AP}^b_{75}$} & {\bf mIoU}           & {\bf $\text{AP}^b$} & {\bf $\text{AP}^b_{50}$} & {\bf $\text{AP}^b_{75}$} & {\bf $\text{AP}^m$} & {\bf $\text{AP}^m_{50}$} & {\bf $\text{AP}^m_{75}$} & mIoU & mIoU \\
            \midrule
            DINO(Swin)           & 51.4                                         & 80.4                      & 56.0                     & 73.6                 & 40.2                & 62.3                     & 43.9                     & 37.6                & 59.3                     & 40.4                     & 78.0 & 62.1 \\
            DINO(Swin) + \putalg & 53.0                                         & 81.0                      & 57.8                     & 75.7                 & 41.0                & 62.9                     & 44.8                     & 38.0                & 59.9                     & 40.9                     & 78.1 & 63.1 \\
            \bottomrule
        \end{tabular}
    \end{adjustbox}
    % \vspace{-3mm}
    \caption{{\small {\bf Results for the Swin transformer backbone pretrained with the DINO framework.} The models are pretrained on the ImageNet1K dataset for 300 epochs. \putalg loss improves the baseline consistently across datasets and tasks. \todo{Include \ours results.} }}
    % \vspace{-2mm}
    \label{tab:swin}
\end{table*}

\customparagraph{Ablation on Learning Rate.}
\todo{[SUPPLEMENTAL] show performance vs lr}

\begin{table}
    \centering
    \caption{\textbf{Ablation studies}}

    \begin{subtable}[t]{0.3\textwidth}
        \caption{\small {\bf learning rate}.}
        \label{tab:abl_lr}
        \centering\begin{tabular}{l c c}
            \toprule
            {lr} & { VOC} & { COCO} \\
            \midrule
            0.3  & 58.9   & 42.0    \\
            0.5  & 59.6   & 42.0    \\
            1.0  & 59.2   & 41.7    \\
        \end{tabular}
    \end{subtable}
    \begin{subtable}[t]{0.3\textwidth}
        \caption{\small {\bf Momentum}.}
        \label{tab:abl_mom}
        \centering\begin{tabular}{l c c}
            \toprule
            {Mom.} & { VOC} & { COCO} \\
            \midrule
            0.99   & 59.1   & 41.3    \\
            0.996  & 58.4   & 41.6    \\
            0.999  & 56.6   & 40.4    \\
        \end{tabular}
    \end{subtable}
    \begin{subtable}[t]{0.3\textwidth}
        \caption{\small {\bf Training image-size}.}
        \label{tab:abl_mom}
        \centering\begin{tabular}{l c c}
            \toprule
            {Im-size} & { VOC} & { COCO} \\
            \midrule
            224$\times$224   & 58.9   & 42.0    \\
            160$\times$160   & 58.4   & 41.6    \\
        \end{tabular}
    \end{subtable}
\end{table}

\customparagraph{Ablation on Momentum.}
\todo{[SUPPLEMENTAL] show performance vs momentum}

\customparagraph{Ablation on Image-size.}
\todo{[SUPPLEMENTAL] show performance vs image-size}

\customparagraph{Ablation on Batch-size.}
\todo{[SUPPLEMENTAL] show performance vs batch-size}

\customparagraph{Pretraining on Non-object-centric Dataset.}

\todo{[SUPPLEMENTAL] Show results for Self-supervised learning on COCO}

\customparagraph{Object Detection and Instance Segmentation.}
For object detection on COCO, we adopt faster RCNN \cite{ren2016fasterrcnn} and RetinaNet \cite{lin2017focalretina} with FPN \cite{lin2017featurefpn} network. We finetune all layers with Sync BatchNorm for 90k iterations on COCO \texttt{train2017} set and evaluate on COCO \texttt{val2017} set. We use the Detectron2 framework \cite{wu2019detectron2} for implementation.  Table \ref{tab:coco_retina} shows object detection results on COCO for our method and other approaches in the literature. Note that ReSim, SoCo, and SCRL use region proposal networks during pretraining on ImageNet, hence, these approaches are not exactly comparable to ours. Our model is more similar with methods like DetCo, DenseCL, and PixPro.  We achieve 40.6 AP for object detection tasks outperforming the second best method SCRL \cite{roh2021spatiallyscrl} by a significant 1.6\% with only 400 epoch (vs 1000 epoch for SCRL). We outperform the baseline BYOL by a huge margin of 5.1\% AP improvement.

In Table \ref{tab:coco_mrcnn}, we report object detection and instance segmentation results on the COCO dataset using the Mask-RCNN framework \cite{he2017maskrcnn} with the ResNet50-FPN backbone. We follow the $1\times$ schedule; results for the $2\times$ schedule are reported in the supplemental materials. Table \ref{tab:coco_mrcnn} reports the detection and instance segmentation performance on COCO. Our method outperforms the BYOL pretrained backbone by 1.3\% AP for object detection and 1.2\% AP for instance segmentation. For object detection, we achieve comparable results with the state-of-the-art methods. 
\sudipta{I have no idea where these numbers 1.3\% and 1.2\% came from. Please be specific about what metric you are talking about. State the relevant values from the table here. be clear.}
SoCo \cite{wei2021aligningsoco} outperforms our method only for object detection on COCO for Mask-RCNN R50-FPN backbone. \sudipta{Why are you calling FPN a backbone?}
However, SoCo is a region-based approach that consists of FPN and RoIAlighn \cite{he2017maskrcnn} networks after the ResNet-50 backbone during pretraining on the ImageNet dataset. Our approach is much simpler and faster to train as it does not require extra region proposal network to produce candidate regions for measuring local consistency.
\sudipta{Table 1 has a lot of numbers, but the text does a poor job discussing the results.}
